# Supplementary material for: Steady state propulsion of isotropic active colloids along a wall
Source: arXiv:2209.07371 ancillary file (2022-09-15)
Supplement: Supplementary file 1 [file main_SI.pdf]

# Supplementary material for "Steady state propulsion of isotropic active colloids along a wall"

Nikhil Desai and Sébastien Michelin

## 1 Expansion of $(\mathbf{u},\ c)$ in non-axisymmetric, bispherical harmonics

The problem geometry is conveniently tackled in a bispherical coordinate system. This requires expressing the flow and solute concentration fields in terms of bispherical harmonic basis functions.

The expansions of the various components of $\mathbf{u}$ are [1]:

$$u_z\left(\xi,\mu,\phi\right)=\frac{z}{2a}\Gamma^{1/2}\sum_{m=0}^{\infty}\sum_{n=m}^{\infty}\left[A_n^m\frac{\sinh\left\{(n+1/2)\lambda\xi\right\}}{\sinh\left\{(n+1/2)\lambda\right\}}+B_n^m\frac{\cosh\left\{(n+1/2)\lambda\xi\right\}}{\cosh\left\{(n+1/2)\lambda\right\}}\right]N_n^m\left(\mu\right)\cos\left(m\phi\right)$$
$$+\Gamma^{1/2}\sum_{m=0}^{\infty}\sum_{n=m}^{\infty}C_n^m\frac{\sinh\left\{(n+1/2)\lambda\xi\right\}}{\sinh\left\{(n+1/2)\lambda\right\}}N_n^m\left(\mu\right)\cos\left(m\phi\right), \qquad (1)$$

$$u_\rho\left(\xi,\mu,\phi\right)=\frac{\rho}{2a}\Gamma^{1/2}\sum_{m=0}^{\infty}\sum_{n=m}^{\infty}\left[A_n^m\frac{\sinh\left\{(n+1/2)\lambda\xi\right\}}{\sinh\left\{(n+1/2)\lambda\right\}}+B_n^m\frac{\cosh\left\{(n+1/2)\lambda\xi\right\}}{\cosh\left\{(n+1/2)\lambda\right\}}\right]N_n^m\left(\mu\right)\cos\left(m\phi\right)$$
$$+\Gamma^{1/2}\sum_{n=1}^{\infty}\left[E_n^0\frac{\sinh\left\{(n+1/2)\lambda\xi\right\}}{\sinh\left\{(n+1/2)\lambda\right\}}+F_n^0\frac{\cosh\left\{(n+1/2)\lambda\xi\right\}}{\cosh\left\{(n+1/2)\lambda\right\}}\right]N_n^1\left(\mu\right)$$
$$+\frac{1}{2}\sum_{m=1}^{\infty}\left\{\gamma_m\left(\xi,\mu\right)+\chi_m\left(\xi,\mu\right)\right\}\cos\left(m\phi\right), \qquad (2)$$

and,

$$u_\phi\left(\xi,\mu,\phi\right)=\frac{1}{2}\sum_{m=1}^{\infty}\left\{\gamma_m\left(\xi,\mu\right)-\chi_m\left(\xi,\mu\right)\right\}\sin\left(m\phi\right), \qquad (3)$$

where, the functions $\gamma_m\left(\xi,\mu\right)$ and $\chi_m\left(\xi,\mu\right)$ in Eqs. (2) and (3) are given by:

$$\gamma_m\left(\xi,\mu\right)=\Gamma^{1/2}\sum_{n=m+1}^{\infty}\left[E_n^m\frac{\sinh\left\{(n+1/2)\lambda\xi\right\}}{\sinh\left\{(n+1/2)\lambda\right\}}+F_n^m\frac{\cosh\left\{(n+1/2)\lambda\xi\right\}}{\cosh\left\{(n+1/2)\lambda\right\}}\right]N_n^{m+1}\left(\mu\right),$$
$$\chi_m\left(\xi,\mu\right)=\Gamma^{1/2}\sum_{n=m-1}^{\infty}\left[G_n^m\frac{\sinh\left\{(n+1/2)\lambda\xi\right\}}{\sinh\left\{(n+1/2)\lambda\right\}}+H_n^m\frac{\cosh\left\{(n+1/2)\lambda\xi\right\}}{\cosh\left\{(n+1/2)\lambda\right\}}\right]N_n^{m-1}\left(\mu\right).$$
$$(4)$$

In the above expansions, the constants $a$ and $\lambda$ are functions of the height $d_p$ of the active particle from the rigid wall (see Fig. 1 in the main manuscript):

$$
\begin{aligned}
a &= \sqrt{d_p(d_p+2)}, \\
\lambda &= \cosh^{-1}(d_p+1),
\end{aligned} \tag{5}
$$

where $\lambda$ is defined such that $\xi = 1$ corresponds to the surface of the particle. $\xi = 0$, on the other hand, corresponds to the surface of the rigid wall.

The bispherical harmonic expansion for the solute concentration is of the form,

$$
c(\xi, \mu, \phi) = \Gamma^{1/2} \sum_{k=0}^{\infty} \sum_{l=k}^{\infty} c_l^k(\xi) N_l^k(\mu) \cos(k\phi). \tag{6}
$$

It will be useful to also write down the expression for $\nabla c$, given by,

$$
\begin{aligned}
\nabla c = &\sum_{k=0}^{\infty} \sum_{l=k}^{\infty} \left\{ \frac{\Gamma^{3/2}}{a\lambda} \frac{dc_l^k}{d\xi} N_l^k(\mu) + \frac{\Gamma^{1/2} \sinh(\lambda\xi)}{2a} N_l^k(\mu)\, c_l^k(\xi) \right\} \cos(k\phi) \mathbf{e}_\xi \\
&+ \sum_{k=0}^{\infty} \sum_{l=k}^{\infty} \left\{ \frac{\Gamma^{3/2}\sqrt{1-\mu^2}}{a} \frac{dN_l^k}{d\mu} - \frac{\Gamma^{1/2}\sqrt{1-\mu^2}}{2a} N_l^k(\mu) \right\} c_l^k(\xi) \cos(k\phi) \mathbf{e}_\mu \\
&+ \sum_{k=0}^{\infty} \sum_{l=k}^{\infty} - \frac{k\Gamma^{3/2}}{a\sqrt{1-\mu^2}} N_l^k(\mu) c_l^k(\xi) \sin(k\phi) \mathbf{e}_\phi.
\end{aligned} \tag{7}
$$

In the above equations, $N_n^m(\mu)$ are the *fully normalized* associated Legendre polynomials, related to the non-normalized associated Legendre polynomials as:

$$
\begin{aligned}
N_n^m(\mu) &= a_n^m P_n^m(\mu), \\
&= (-1)^m \left\{ \frac{(n+1/2)(n-m)!}{(n+m)!} \right\}^{\frac{1}{2}} P_n^m(\mu).
\end{aligned} \tag{8}
$$

Note that the $\cos(\phi)$ dependence of $(u_r, u_z, c)$ and the $\sin(\phi)$ dependence of $u_\phi$, comes from the consideration of steady state swimming in the particle frame, under which the particle is swimming parallel to the wall in the lab frame. In addition, the fluid velocity expansions are defined such that the wall impermeability condition, $u_z(\xi = 0, \mu, \phi) = 0$, is automatically satisfied.

# 2 Solution methodology

The steady state advection-diffusion equation (Eqn. (9) in the main manuscript) needs to be solved along with the boundary conditions for $c$ (Eqns. (2) in the main manuscript), and boundary-driven Stokes flow problem (Eqns. (4) to (8) in the main manuscript). The solution methodology requires expanding the fields ($\mathbf{u}$, $c$) in bi-spherical harmonic series (Sec. 1), substituting in the advection-diffusion equation, and projecting the resulting equation onto $N_j^i(\mu)\cos(i\phi)/\Gamma$,

i.e., the orthogonal bases of the bi-spherical expansion. This yields a family of coupled, non-linear, ordinary differential equations that can be formally written as:

$$\mathbf{A}^0\left(\mathcal{U}_H\right)\cdot\mathbf{C}+\mathbf{A}^1\left(\mathcal{U}_H\right)\cdot\frac{d\mathbf{C}}{d\xi}=\frac{1}{\mathrm{Pe}}\left\{\mathbf{D}^0\cdot\mathbf{C}+\mathbf{D}^2\cdot\frac{d^2\mathbf{C}}{d\xi^2}\right\}, \tag{9}$$

where,

$$\mathbf{C}\equiv\left[\left\{c_0^0(\xi),...,c_N^0(\xi)\right\},\ \left\{c_1^1(\xi),...,c_N^1(\xi)\right\},\ \left\{c_m^m(\xi),...,c_N^m(\xi)\right\},\ ...\right],$$

are the unknown functions in the bispherical harmonic expansion of $c$ that need to be determined (see Eqn. (6)). In Eqn. (9), the terms involving $\mathbf{D}^0$ and $\mathbf{D}^2$ abbreviate the projection of the diffusion term $\nabla^2 c$. $\mathbf{D}^0$ and $\mathbf{D}^2$ are fourth order tensors depending only on $\xi$, and their values are given in Sec. 3.

Next, the terms involving $\mathbf{A}^0$ and $\mathbf{A}^1$ abbreviate the projection of the advection term $(\mathbf{u}-\mathbf{U})\cdot\nabla c$. These are complicated summations that are explicitly written out in Sec. 4. In addition,

$$\mathcal{U}_H\equiv\left[A_n^m,\ B_n^m,\ C_n^m,\ E_n^m,\ F_n^m,\ G_n^m,\ H_n^m;\ U_x\right],$$

is a short-hand for: (i) the unknown coefficients in the bispherical harmonic expansions of the fluid velocity, $\mathbf{u}=u_r\mathbf{e}_r+u_z\mathbf{e}_z+u_\phi\mathbf{e}_\phi$ (see Eqns. (1) to (3)), and, (ii) the particle's swimming speed, $U_x$.

The flow coefficients, $\mathcal{U}_H$ are expressible as a linear function of the concentration modes, $\mathbf{C}$, via orthogonal projections of the continuity equation and velocity boundary conditions at the wall and the surface of the particle (see Sec. 5). Therefore, we can write $\mathcal{U}_H\equiv\mathbf{H}\cdot\mathbf{C}$, where $\mathbf{H}$ is a linear operator whose entries are defined in Section 5, and we see that Eqn. (9) is *non-linear* in $\mathbf{C}$.

Eqn. (9) is complemented by the projection of the boundary conditions for $c$ (Eqns. 2 in the main manuscript), on to the orthogonal modes $N_j^i(\mu)\cos(i\phi)$:

$$\left.-\frac{j-i}{2j-1}\frac{dc_{j-1}^i}{d\xi}+\frac{dc_j^i}{d\xi}-\frac{j+i+1}{2j+3}\frac{dc_{j+1}^i}{d\xi}\right|_{\xi=0}=0,\ \text{for all } i, \tag{10}$$

and,

$$\begin{aligned}&\left(-a_{j-1}^i\frac{j-i}{2j-1}\frac{dc_{j-1}^i}{d\xi}-a_{j+1}^i\frac{j+i+1}{2j+3}\frac{dc_{j+1}^i}{d\xi}\right.\\&\left.\left.+a_j^i\frac{\lambda\sinh\lambda}{2}c_j^i+a_j^i\cosh\lambda\frac{dc_j^i}{d\xi}\right)\right|_{\xi=1}=\sqrt{2}a\lambda\mathrm{e}^{-\lambda(j+1/2)},\ \text{for } i=0,\end{aligned} \tag{11}$$

$$\begin{aligned}&\left(-a_{j-1}^i\frac{j-i}{2j-1}\frac{dc_{j-1}^i}{d\xi}-a_{j+1}^i\frac{j+i+1}{2j+3}\frac{dc_{j+1}^i}{d\xi}\right.\\&\left.\left.+a_j^i\frac{\lambda\sinh\lambda}{2}c_j^i+a_j^i\cosh\lambda\frac{dc_j^i}{d\xi}\right)\right|_{\xi=1}=0,\ \text{for } i\geq 1.\end{aligned} \tag{12}$$

Eqns. (9) to (12) can be represented as a non-linear system in $\mathbf{C}$,

$$\mathcal{N}\left(\mathbf{H} \cdot \mathbf{C}, \mathbf{C}\right) = \mathbf{R}, \tag{13}$$

where the only non-homogeneity in the system comes from the right hand side of Eqn. (12) for $i = 0$. Eqn. (13) is solved using the iterative scheme,

$$\mathcal{N}\left(\mathbf{H} \cdot \mathbf{C}^n, \mathbf{C}^{n+1}\right) = -\mathcal{N}\left(\mathbf{H} \cdot \mathbf{C}^n, \mathbf{C}^n\right) + \mathbf{R}, \tag{14}$$

where, the super-script $n$ refers to the values at the $n$-th iteration. Additionally,

1. the $\xi$-derivatives, $\left(d\mathbf{C}/d\xi, d^2\mathbf{C}/d\xi^2\right)$, are discretized using second-order accurate, centered finite differences over $P$ equi-spaced points between $\xi = 0, 1$, and,

2. the expansions for $(c, \mathbf{u})$ are truncated at an appropriate number of polar and azimuthal modes.

At a prescribed $(d_p, \mathrm{Pe})$, the iterator is initiated with $[\mathbf{C},\ \mathcal{U}_H]$ corresponding to the stationary, axisymmetric, hovering state that has been discussed in detail in Ref. [2]. A small non-axisymmetry is imposed by initializing $U_x = 10^{-3}$. The iterator is stopped if the relative error in $U_x$ goes below 0.1%. The case of $d_p \gg 1$ acts as a validation of the present numerical method, where we recover the results of Ref. [3] for the motion of an isotropic, phoretic particle in an unbounded fluid (see Fig. 2a in main manuscript).

In our computations, we truncated the summations of eqns. (1) to (3) and eqn. (6) at different numbers of azimuthal modes (say $N$), and polar modes (say $M$), depending on the propulsion separation, $d_p$. This, along with the $\xi$-discretization of the modes $c_n^m(\xi)$, leads to a matrix system of $(M + 1)(N + 1 - M/2)P$ unknowns, which must be constructed and inverted in each iteration described by eqn. (14) until a converged value of the translation speed, $U_x$, is obtained. The independence of the results on the modal resolution was checked by increasing the number of modes in increments of $(\Delta N = 5, \Delta M = 2)$, until there was $< 1\%$ change in the converged value of the swimming speed, $U_x$. The highest resolution corresponded to the case of $(F^{ext} = 9.13, \mathrm{Pe} = 8)$ and $d_p \approx 0.4$, with there being $\approx 1\%$ relative error in $U_x$ between $(N = 30, M = 4)$ and $(N = 35, M = 8)$. The lowest resolution corresponded to the case of $(F^{ext} = 1.19, \mathrm{Pe} = 4)$ and $d_p \approx 1.5$, with there being $< 1\%$ relative error in $U_x$ between $(N = 15, M = 6)$ and $(N = 25, M = 10)$. For the $\xi$-discretization, we found that $P = 100$ gives an accurate enough resolution of the derivative terms in eqn. (9), with the difference in $U_x$ between $P = 100$ and $P = 150$ being imperceptible.

In the final paragraph of the main manuscript, we mentioned that our numerical method does not allow us to cover a broad range of Péclet numbers, Pe. In the steady swimming regime, the non-linear coupling between the azimuthal and polar concentration modes is strengthened for: (i) large values of Pe, and, (ii) small values of the propulsion separation, $d_p$. An enhanced coupling between the concentration modes thus demands an increase in the number of modes that

need to be retained in the bispherical harmonic expansions (eqns. (1) to (3) and eqn. (6)). For the values of $F^{ext}$ considered in the main manuscript, our computations fail to converge for large Pe, even at the maximum resolution considered ($N = 35, M = 8$). Including even more number of azimuthal and/or polar modes greatly increases the memory and computational time, due to a large increase in the storage of the sixth order 'coupling tensors' $I^{A,kmi}_{lnj}$ to $I^{H,kmi}_{lnj}$ and $I^{pA,kmi}_{lnj}$ to $I^{pH,kmi}_{lnj}$ (see eqns. (22) to (35)). Note that each entry of these tensors is unique and needs to be computed and stored beforehand to prevent inefficient calculations in our iterative procedure. Thus, the computational cost associated with improving the resolution (and thus obtaining convergence) at large Pe becomes prohibitive.

# 3 Projection of the diffusion term

Here, we give expressions for the fourth order 'diffusion tensors', $\mathbf{D}^0$ and $\mathbf{D}^2$, from Eqn. (9). These are obtained after projection of the $\nabla^2 c$ term onto the Legendre mode $N^i_j(\mu)\cos(i\phi)/\Gamma$. Since $\nabla^2 c$ is linear in $c$, the orthogonality of the $\phi$-modes makes it such that *only* the $c^k_l(\xi)$ modes corresponding to $k = i$ (see Eqn. (6)) contribute to the terms $\mathbf{D}^0 \cdot \mathbf{C}$ and $\mathbf{D}^2 \cdot d^2\mathbf{C}/d\xi^2$ in Eqn. 9. The projection of the diffusion term at $\xi = \xi_p$ can be written as,

$$\int_0^{2\pi}\int_{-1}^{1} \frac{\nabla^2 c}{\Gamma} N^i_j(\mu)\cos(i\phi)\, d\mu\, d\phi = \sum_{k=0}^{\infty}\sum_{l=k}^{\infty} c^k_l(\xi_p) \times \left(\mathbf{D}^0\right)^{ki}_{lj} + \sum_{k=0}^{\infty}\sum_{l=k}^{\infty} \frac{d^2 c^k_l}{d\xi^2} \times \left(\mathbf{D}^2\right)^{ki}_{lj}, \tag{15}$$

where,

$$\left(\mathbf{D}^2\right)^{ki}_{lj} = \mathcal{F}(i)\delta_{ki} \sum_{q=0}^{\infty} \frac{\sqrt{2}}{a^2\lambda^2} \left(\cosh^2(\lambda\xi_p) Q^{0,i}_{qlj} - 2\cosh(\lambda\xi_p) Q^{1,i}_{qlj} + Q^{2,i}_{qlj}\right) \mathrm{e}^{-(q+1/2)\lambda\xi_p}, \tag{16}$$

and,

$$\left(\mathbf{D}^0\right)^{ki}_{lj} = -\lambda^2(l+1/2)^2 \left(\mathbf{D}^2\right)^{ki}_{lj}, \tag{17}$$

where, $\delta_{ki}$ is the Dirac delta, and the pre-factor $\mathcal{F}(i)$ takes care of the $\phi$-integration, such that,

$$\mathcal{F}(i) = \begin{cases} 2\pi, & \text{if } i = 0 \\ \pi, & \text{if } i \geq 1 \end{cases}. \tag{18}$$

The $Q^{x,i}_{qlj}$ tensors in Eqn. (16) are integrals involving Legendre polynomials, given by:

$$Q^{x,i}_{qlj} = \int_{-1}^{1} \mu^x P^0_q(\mu) N^i_l(\mu) N^i_j(\mu)\, d\mu, \tag{19}$$

where $P_q^0(\mu)$ is the *non*-normalized associated Legendre polynomial of zeroth order and degree $q$, and $N_l^i(\mu)$, $N_j^i(\mu)$ are the *fully normalized* associated Legendre polynomials as defined in Eqn. (8).

# 4 Projection of the advection term

## 4.1 Projection of $\mathbf{u} \cdot \nabla c$ onto the family of orthogonal associated Legendre modes

Our aim is to project the advection term, $\mathbf{u} \cdot \nabla c$, onto the family of orthogonal Legendre modes $N_j^i(\mu)\cos(i\phi)/\Gamma$. This leads to evaluation of the integral,

$$\int_0^{2\pi} \int_{-1}^{1} \frac{\mathbf{u} \cdot \nabla c}{\Gamma} N_j^i(\mu) \cos(i\phi)\, d\mu\, d\phi, \tag{20}$$

which is the first contribution to the $\left\{\mathbf{A}^0\left(\mathcal{U}_H\right) \cdot \mathbf{C} + \mathbf{A}^1\left(\mathcal{U}_H\right) \cdot d\mathbf{C}/d\xi\right\}$ term in Eqn. (9) (the second contribution comes from the projection of $-\mathbf{U} \cdot \nabla c$, as shown in Sec. 4.2).

When the advection term at $\xi = \xi_p$ is projected onto a mode $N_j^i(\mu)\cos(i\phi)/\Gamma$, the integral in eqn. (20) can be written as:

$$\begin{gathered}
\sum_{k=0}^{\infty}\sum_{l=k}^{\infty} c_l^k\left(\xi_p\right) \times \left\{\begin{array}{l}
\sum\limits_{m=0}^{\infty}\sum\limits_{n=m}^{\infty}\left(A_n^m I_{lnj}^{A,kmi} + B_n^m I_{lnj}^{B,kmi} + C_n^m I_{lnj}^{C,kmi}\right) + \\
\sum\limits_{m=1}^{\infty}\sum\limits_{n=m+1}^{\infty}\left(E_n^m I_{lnj}^{E,kmi} + F_n^m I_{lnj}^{F,kmi}\right) + \\
\sum\limits_{m=1}^{\infty}\sum\limits_{n=m-1}^{\infty}\left(G_n^m I_{lnj}^{G,kmi} + H_n^m I_{lnj}^{H,kmi}\right)
\end{array}\right\} \\
+ \\
\sum_{l=i}^{\infty} c_l^i\left(\xi_p\right) \times \left\{\sum_{n=1}^{\infty}\left(E_n^0 J_{lnj}^{E,i1i} + F_n^0 J_{lnj}^{F,i1i}\right)\right\} \\
+ \\
\sum_{k=0}^{\infty}\sum_{l=k}^{\infty} \frac{dc_l^k}{d\xi} \times \left\{\begin{array}{l}
\sum\limits_{m=0}^{\infty}\sum\limits_{n=m}^{\infty}\left(A_n^m I_{lnj}^{pA,kmi} + B_n^m I_{lnj}^{pB,kmi} + C_n^m I_{lnj}^{pC,kmi}\right) + \\
\sum\limits_{m=1}^{\infty}\sum\limits_{n=m+1}^{\infty}\left(E_n^m I_{lnj}^{pE,kmi} + F_n^m I_{lnj}^{pF,kmi}\right) + \\
\sum\limits_{m=1}^{\infty}\sum\limits_{n=m-1}^{\infty}\left(G_n^m I_{lnj}^{pG,kmi} + H_n^m I_{lnj}^{pH,kmi}\right)
\end{array}\right\} \\
+ \\
\sum_{l=i}^{\infty} \frac{dc_l^i}{d\xi} \times \left\{\sum_{n=1}^{\infty}\left(E_n^0 J_{lnj}^{pE,i1i} + F_n^0 J_{lnj}^{pF,i1i}\right)\right\}
\end{gathered} \tag{21}$$

In eqn. (21), the factors of $c_l^k(\xi_p)$ and $c_l^i(\xi_p)$ contribute to the $\mathbf{A}^0(\mathcal{U}_H)$ term in Eqn. (9); and the factors of $dc_l^k(\xi_p)/d\xi$ and $dc_l^i(\xi_p)/d\xi$ contribute to the $\mathbf{A}^1(\mathcal{U}_H)$ term in Eqn. (9). The sixth order tensors $I_{lnj}^{A,kmi}$ to $I_{lnj}^{H,kmi}$, and $I_{lnj}^{pA,kmi}$ to $I_{lnj}^{pH,kmi}$ are functions of $\xi$ alone and involve integrations of various combinations

of the fully normalized associated Legendre polynomials and their derivatives. These are detailed below:

$$I_{lnj}^{A,kmi}(\xi_p) = \frac{1}{2a}\frac{\sinh\{(n+1/2)\lambda\xi_p\}}{\sinh\{(n+1/2)\lambda\}}\left[-\frac{1}{2}\mathscr{A}_{lnj}^{0,kmi} - \frac{\cosh(\lambda\xi_p)}{2}\mathscr{A}_{lnj}^{1,kmi} + \cosh(\lambda\xi_p)\mathscr{B}_{lnj}^{0,kmi}\right] \tag{22}$$

$$I_{lnj}^{B,kmi}(\xi_p) = I_{lnj}^{A,kmi}(\xi_p) \times \frac{\tanh\{(n+1/2)\lambda\}}{\tanh\{(n+1/2)\lambda\xi_p\}} \tag{23}$$

$$I_{lnj}^{C,kmi}(\xi_p) = \frac{1}{2a}\frac{\sinh\{(n+1/2)\lambda\xi_p\}}{\sinh\{(n+1/2)\lambda\}}\left[-\sinh(\lambda\xi_p)\mathscr{A}_{lnj}^{1,kmi} + 2\sinh(\lambda\xi_p)\mathscr{B}_{lnj}^{0,kmi}\right] \tag{24}$$

$$\begin{aligned} I_{lnj}^{E,kmi}(\xi_p) = {} & \frac{1}{2a}\frac{\sinh\{(n+1/2)\lambda\xi_p\}}{\sinh\{(n+1/2)\lambda\}}\left[-\frac{\cosh(\lambda\xi_p)}{2}\mathscr{C}_{lnj}^{0,kmi} + \mathscr{D}_{lnj}^{0,kmi} - \cosh(\lambda\xi_p)\mathscr{D}_{lnj}^{1,kmi}\right] \\ & - \frac{k}{2a}\frac{\sinh\{(n+1/2)\lambda\xi_p\}}{\sinh\{(n+1/2)\lambda\}}\left[\cosh(\lambda\xi_p)\mathscr{E}_{lnj}^{0,kmi} - \mathscr{E}_{lnj}^{1,kmi}\right] \end{aligned} \tag{25}$$

$$I_{lnj}^{F,kmi}(\xi_p) = I_{lnj}^{E,kmi}(\xi_p) \times \frac{\tanh\{(n+1/2)\lambda\}}{\tanh\{(n+1/2)\lambda\xi_p\}} \tag{26}$$

$$\begin{aligned} I_{lnj}^{G,kmi}(\xi_p) = {} & \frac{1}{2a}\frac{\sinh\{(n+1/2)\lambda\xi_p\}}{\sinh\{(n+1/2)\lambda\}}\left[-\frac{\cosh(\lambda\xi_p)}{2}\mathscr{F}_{lnj}^{0,kmi} + \mathscr{G}_{lnj}^{0,kmi} - \cosh(\lambda\xi_p)\mathscr{G}_{lnj}^{1,kmi}\right] \\ & + \frac{k}{2a}\frac{\sinh\{(n+1/2)\lambda\xi_p\}}{\sinh\{(n+1/2)\lambda\}}\left[\cosh(\lambda\xi_p)\mathscr{H}_{lnj}^{0,kmi} - \mathscr{H}_{lnj}^{1,kmi}\right] \end{aligned} \tag{27}$$

$$I_{lnj}^{H,kmi}(\xi_p) = I_{lnj}^{G,kmi}(\xi_p) \times \frac{\tanh\{(n+1/2)\lambda\}}{\tanh\{(n+1/2)\lambda\xi_p\}} \tag{28}$$

$$I_{lnj}^{pA,kmi}(\xi_p) = -\frac{\sinh(\lambda\xi_p)}{2\lambda a}\frac{\sinh\{(n+1/2)\lambda\xi_p\}}{\sinh\{(n+1/2)\lambda\}}\mathscr{A}_{lnj}^{1,kmi} \tag{29}$$

$$I_{lnj}^{pB,kmi}(\xi_p) = I_{lnj}^{pA,kmi}(\xi_p) \times \frac{\tanh\{(n+1/2)\lambda\}}{\tanh\{(n+1/2)\lambda\xi_p\}} \tag{30}$$

$$I_{lnj}^{pC,kmi}(\xi_p) = \frac{1}{\lambda a}\frac{\sinh\{(n+1/2)\lambda\xi_p\}}{\sinh\{(n+1/2)\lambda\}}\left[\mathscr{A}_{lnj}^{0,kmi} - \cosh(\lambda\xi_p)\mathscr{A}_{lnj}^{1,kmi}\right] \tag{31}$$

$$I_{lnj}^{pE,kmi}(\xi_p) = -\frac{\sinh(\lambda\xi_p)}{2\lambda a}\frac{\sinh\{(n+1/2)\lambda\xi_p\}}{\sinh\{(n+1/2)\lambda\}}\mathscr{C}_{lnj}^{0,kmi} \tag{32}$$

$$I_{lnj}^{pF,kmi}(\xi_p) = I_{lnj}^{pE,kmi}(\xi_p) \times \frac{\tanh\{(n+1/2)\lambda\}}{\tanh\{(n+1/2)\lambda\xi_p\}} \tag{33}$$

$$I_{lnj}^{pG,kmi}\left(\xi_p\right) = -\frac{\sinh\left(\lambda\xi_p\right)}{2\lambda a}\frac{\sinh\left\{\left(n+1/2\right)\lambda\xi_p\right\}}{\sinh\left\{\left(n+1/2\right)\lambda\right\}}\mathscr{F}_{lnj}^{0,kmi} \tag{34}$$

$$I_{lnj}^{pH,kmi}\left(\xi_p\right) = I_{lnj}^{pG,kmi}\left(\xi_p\right) \times \frac{\tanh\left\{\left(n+1/2\right)\lambda\right\}}{\tanh\left\{\left(n+1/2\right)\lambda\xi_p\right\}} \tag{35}$$

In the eqns. (22) to (35), the 'script' letters denote numerical values obtained via following integrations:

$$\mathscr{A}_{lnj}^{x,kmi} = \left\langle \mu^x N_l^k(\mu) N_n^m(\mu)\cos(k\phi)\cos(m\phi)\right\rangle, \tag{36}$$

$$\mathscr{B}_{lnj}^{x,kmi} = \left\langle \mu^x(1-\mu^2)\frac{dN_l^k}{d\mu}N_n^m(\mu)\cos(k\phi)\cos(m\phi)\right\rangle, \tag{37}$$

$$\mathscr{C}_{lnj}^{x,kmi} = \left\langle \mu^x\sqrt{1-\mu^2}N_l^k(\mu)N_n^{m+1}(\mu)\cos(k\phi)\cos(m\phi)\right\rangle, \tag{38}$$

$$\mathscr{D}_{lnj}^{x,kmi} = \left\langle \mu^x\sqrt{1-\mu^2}\frac{dN_l^k}{d\mu}N_n^{m+1}(\mu)\cos(k\phi)\cos(m\phi)\right\rangle, \tag{39}$$

$$\mathscr{E}_{lnj}^{x,kmi} = \left\langle \mu^x\frac{N_l^k(\mu)N_n^{m+1}(\mu)}{\sqrt{1-\mu^2}}\sin(k\phi)\sin(m\phi)\right\rangle, \tag{40}$$

$$\mathscr{F}_{lnj}^{x,kmi} = \left\langle \mu^x\sqrt{1-\mu^2}N_l^k(\mu)N_n^{m-1}(\mu)\cos(k\phi)\cos(m\phi)\right\rangle, \tag{41}$$

$$\mathscr{G}_{lnj}^{x,kmi} = \left\langle \mu^x\sqrt{1-\mu^2}\frac{dN_l^k}{d\mu}N_n^{m-1}(\mu)\cos(k\phi)\cos(m\phi)\right\rangle, \tag{42}$$

$$\mathscr{H}_{lnj}^{x,kmi} = \left\langle \mu^x\frac{N_l^k(\mu)N_n^{m-1}(\mu)}{\sqrt{1-\mu^2}}\sin(k\phi)\sin(m\phi)\right\rangle, \tag{43}$$

where the angle brackets denote the projection onto the Legendre mode $N_j^i(\mu)\cos(i\phi)$:

$$\left\langle f\left(\mu,\phi\right)\right\rangle = \int_0^{2\pi}\int_{-1}^{1} f\left(\mu,\phi\right)N_j^i(\mu)\cos(i\phi)\,d\mu\,d\phi. \tag{44}$$

Similar to the sixth order tensors in eqn. (21), the fourth order tensors $J_{lnj}^{E/F,\mathrm{i1i}}$ and $J_{lnj}^{pE/pF,\mathrm{i1i}}$, are functions of $\xi$ alone and involve various combinations of the fully normalized associated Legendre polynomials and their derivatives. These are given by:

$$J_{lnj}^{E,i1i}\left(\xi_p\right) = \frac{1}{2a}\frac{\sinh\left\{\left(n+1/2\right)\lambda\xi_p\right\}}{\sinh\left\{\left(n+1/2\right)\lambda\right\}}\left[-\cosh\left(\lambda\xi_p\right)\mathscr{J}_{lnj}^{0,i} + 2\mathscr{K}_{lnj}^{0,i} - 2\cosh\left(\lambda\xi_p\right)\mathscr{K}_{lnj}^{1,i}\right] \tag{45}$$

$$J_{lnj}^{F,i1i}\left(\xi_p\right) = J_{lnj}^{E,i1i}\left(\xi_p\right) \times \frac{\tanh\left\{\left(n+1/2\right)\lambda\right\}}{\tanh\left\{\left(n+1/2\right)\lambda\xi_p\right\}} \tag{46}$$

$$J_{lnj}^{pE,i1i}(\xi_p) = -\frac{\sinh(\lambda\xi_p)}{\lambda a}\frac{\sinh\{(n+1/2)\lambda\xi_p\}}{\sinh\{(n+1/2)\lambda\}}\mathscr{I}_{lnj}^{0,i} \tag{47}$$

$$J_{lnj}^{pF,i1i}(\xi_p) = J_{lnj}^{pE,i1i}(\xi_p) \times \frac{\tanh\{(n+1/2)\lambda\}}{\tanh\{(n+1/2)\lambda\xi_p\}} \tag{48}$$

Again, the 'script' letters denote numerical values obtained via following integrations:

$$\mathscr{I}_{lnj}^{x,i} = \begin{cases} 2\pi\int\limits_{-1}^{1}\mu^x\sqrt{1-\mu^2}N_l^i(\mu)\,N_n^1(\mu)\,N_j^i(\mu)d\mu,\ i=0 \\ \pi\int\limits_{-1}^{1}\mu^x\sqrt{1-\mu^2}N_l^i(\mu)\,N_n^1(\mu)\,N_j^i(\mu)d\mu,\ i>0 \end{cases}, \tag{49}$$

and,

$$\mathscr{K}_{lnj}^{x,i} = \begin{cases} 2\pi\int\limits_{-1}^{1}\mu^x\sqrt{1-\mu^2}\frac{dN_l^i}{d\mu}N_n^1(\mu)\,N_j^i(\mu)d\mu,\ i=0 \\ \pi\int\limits_{-1}^{1}\mu^x\sqrt{1-\mu^2}\frac{dN_l^i}{d\mu}N_n^1(\mu)\,N_j^i(\mu)d\mu,\ i>0 \end{cases}. \tag{50}$$

### 4.2 Projection of $-\mathbf{U}\cdot\nabla c$ onto the family of orthogonal associated Legendre modes

Next, we aim to project the advection term, $-\mathbf{U}\cdot\nabla c$, onto the family of orthogonal Legendre modes $N_j^i(\mu)\cos(i\phi)/\Gamma$. This leads to evaluation of the integral,

$$-\int_0^{2\pi}\int_{-1}^{1}\frac{\mathbf{U}\cdot\nabla c}{\Gamma}N_j^i(\mu)\cos(i\phi)\,d\mu\,d\phi, \tag{51}$$

which is the second contribution to the $\left\{\mathbf{A}^0(\mathcal{U}_H)\cdot\mathbf{C}+\mathbf{A}^1(\mathcal{U}_H)\cdot d\mathbf{C}/d\xi\right\}$ term in Eqn. (9) (the first contribution comes from the projection of $\mathbf{u}\cdot\nabla c$, as shown in Sec. 4.1). Substituting,

$$\mathbf{U} = U_x\cos(\phi)\mathbf{e}_r - U_x\sin(\phi)\mathbf{e}_\phi, \tag{52}$$

and $\nabla c$ (from Eqns. (6) and (7)) into Eqn. (51), we obtain:

$$\begin{gathered} U_x\sum_{k=0}^{\infty}\sum_{l=k}^{\infty}c_l^k(\xi_p)\times\left\langle f_r^0(\xi,\mu,\phi;k,l)+f_\phi^0(\xi,\mu,\phi;k,l)\right\rangle \\ + \\ U_x\sum_{k=0}^{\infty}\sum_{l=k}^{\infty}\frac{dc_l^k}{d\xi}\times\left\langle f_r^1(\xi,\mu,\phi;k,l)\right\rangle, \end{gathered} \tag{53}$$

where, once again, the angled brackets denote the projection described in Eqn. (44). The functions $f_r^{0,1}$ and $f_\phi^1$ are defined below:

$$f_r^0(\xi,\mu,\phi;k,l) = \frac{\sqrt{1-\mu^2}}{a\Gamma^{1/2}}\left\{-N_l^k(\mu)\frac{\cosh(\lambda\xi)}{2} + (1-\mu\cosh(\lambda\xi))\frac{dN_l^k}{d\mu}\right\}\cos(\phi)\cos(k\phi) \tag{54}$$

$$f_r^1(\xi,\mu,\phi;k,l) = -\frac{\sinh(\lambda\xi)}{\lambda a\Gamma^{1/2}}\sqrt{1-\mu^2}N_l^k(\mu)\cos(\phi)\cos(k\phi) \tag{55}$$

$$f_\phi^0(\xi,\mu,\phi;k,l) = \frac{k\Gamma^{1/2}}{a\sqrt{1-\mu^2}}N_l^k(\mu)\sin(\phi)\sin(k\phi) \tag{56}$$

# 5 Linear equations for the velocity coefficients

The coefficients in the expansions of the velocity field are solutions of the linear system of equations obtained via projection of the boundary conditions and the continuity equation onto the Legendre modes $N_n^m(\mu)\cos(m\phi)$. These linear systems are best represented separately for $i=0$ and $i\geq 1$. It is important to note that due to the use of the fully normalized associated Legendre polynomials and the bounded supports for the $\xi$-dependence, the linear equations governing the coefficients in the velocity field expansions are slightly different from those found in classical literature [1, 4], and are summarized next. In what follows, we use the notation,

$$\begin{aligned} Si_n &\equiv \sinh\{(n+1/2)\lambda\}, \\ Co_n &\equiv \cosh\{(n+1/2)\lambda\}, \end{aligned} \tag{57}$$

and,

$$a_n^m = (-1)^m\left\{\frac{(n+1/2)\,(n-m)!}{(n+m)!}\right\}^{\frac{1}{2}}. \tag{58}$$

## 5.1 Axisymmetric components of the velocity coefficients, $m=0$

### 5.1.1 No slip condition at the wall (one equation)

$$\begin{aligned} &-\frac{a_{n-1}^0}{2\,(2n-1)\,Co_{n-1}}B_{n-1}^0 + \frac{a_{n+1}^0}{2\,(2n+3)\,Co_{n+1}}B_{n+1}^0 \\ &-\frac{(n-1)}{(2n-1)}\frac{a_{n-1}^1}{Co_{n-1}}F_{n-1}^0 + \frac{a_n^1}{Co_n}F_n^0 - \frac{(n+2)}{(2n+3)}\frac{a_{n+1}^1}{Co_{n+1}}F_{n+1}^0 = 0 \end{aligned} \tag{59}$$

### 5.1.2 Continuity equation (two equations)

$$
\begin{aligned}
&-\frac{n}{2}\frac{a_{n-1}^{0}}{Si_{n-1}}A_{n-1}^{0}+\frac{5a_{n}^{0}}{2Si_{n}}A_{n}^{0}+\frac{n+1}{2}\frac{a_{n+1}^{0}}{Si_{n+1}}A_{n+1}^{0}\\
&-n\left(n-1\right)\frac{a_{n-1}^{1}}{Si_{n-1}}E_{n-1}^{0}+2n\left(n+1\right)\frac{a_{n}^{1}}{Si_{n}}E_{n}^{0}-\left(n+1\right)\left(n+2\right)\frac{a_{n+1}^{1}}{Si_{n+1}}E_{n+1}^{0}=0
\end{aligned}
\tag{60}
$$

$$
\begin{aligned}
&-\frac{n}{2}\frac{a_{n-1}^{0}}{Co_{n-1}}B_{n-1}^{0}+\frac{5a_{n}^{0}}{2Co_{n}}B_{n}^{0}+\frac{n+1}{2}\frac{a_{n+1}^{0}}{Co_{n+1}}B_{n+1}^{0}\\
&-n\frac{a_{n-1}^{0}}{Si_{n-1}}C_{n-1}^{0}+\left(2n+1\right)\frac{a_{n}^{0}}{Si_{n}}C_{n}^{0}-\left(n+1\right)\frac{a_{n+1}^{0}}{Si_{n+1}}C_{n+1}^{0}\\
&-n\left(n-1\right)\frac{a_{n-1}^{1}}{Co_{n-1}}F_{n-1}^{0}+2n\left(n+1\right)\frac{a_{n}^{1}}{Co_{n}}F_{n}^{0}-\left(n+1\right)\left(n+2\right)\frac{a_{n+1}^{1}}{Co_{n+1}}F_{n+1}^{0}=0
\end{aligned}
\tag{61}
$$

### 5.1.3 Slip boundary condition on particle surface (two equations)

In the following Eqns. (62) and (63) (also in Eqns. (68) and (69)), the notation $c_n^m(1)$ is short-hand for $c_n^m(\xi = 1)$.

$$
\begin{aligned}
&-\frac{a_{n-1}^{0}}{2\left(2n-1\right)}\left(A_{n-1}^{0}+B_{n-1}^{0}\right)+\frac{a_{n+1}^{0}}{2\left(2n+3\right)}\left(A_{n+1}^{0}+B_{n+1}^{0}\right)\\
&-\frac{\left(n-1\right)}{\left(2n-1\right)}a_{n-1}^{1}\left(E_{n-1}^{0}+F_{n-1}^{0}\right)+\cosh\left(\lambda\right)a_{n}^{1}\left(E_{n}^{0}+F_{n}^{0}\right)\\
&-\frac{\left(n+2\right)}{\left(2n+3\right)}a_{n+1}^{1}\left(E_{n+1}^{0}+F_{n+1}^{0}\right)\\
&=\frac{1}{2a}\left\{-a_{n-2}^{0}\frac{\left(n-1\right)}{\left(2n-1\right)}\cosh\left(\lambda\right)c_{n-2}^{0}\left(1\right)-a_{n+2}^{0}\frac{\left(n+2\right)}{\left(2n+3\right)}\cosh\left(\lambda\right)c_{n+2}^{0}\left(1\right)\right.\\
&+a_{n-1}^{0}\frac{1+2\left(n-1\right)\left(1+\cosh^{2}\left(\lambda\right)\right)}{\left(2n-1\right)}c_{n-1}^{0}\left(1\right)\\
&-a_{n+1}^{0}\frac{1-2\left(n+2\right)\left(1+\cosh^{2}\left(\lambda\right)\right)}{\left(2n+3\right)}c_{n+1}^{0}\left(1\right)\\
&\left.-a_{n}^{0}\cosh\left(\lambda\right)\frac{12n^{2}+12n-11}{\left(2n-1\right)\left(2n+3\right)}c_{n}^{0}\left(1\right)\right\}
\end{aligned}
\tag{62}
$$

$$
\begin{aligned}
&a_n^m \frac{\sinh(\lambda)}{2}\left(A_n^m + B_n^m\right) - a_{n-1}^m \frac{(n-m)}{(2n-1)} C_{n-1}^m \\
&+ a_n^m \cosh(\lambda)\, C_n^m - a_{n+1}^m \frac{(n+m+1)}{(2n+3)} C_{n+1}^m \\
&= \frac{\sinh(\lambda)}{2a}\left\{ a_{n-2}^m c_{n-2}^m(1) \frac{(n-m-1)(n-m)}{(2n-1)} - a_{n-1}^m c_{n-1}^m(1) \frac{2\cosh(\lambda)(n-m)(n-1)}{(2n-1)} \right\} \\
&+ \frac{a_n^m \sinh(\lambda)}{a} c_n^m(1) \frac{(-2n^2 - 2n + 1 + 2m^2)}{(2n-1)(2n+3)} \\
&+ \frac{\sinh(\lambda)}{2a}\left\{ a_{n+1}^m c_{n+1}^m(1) \frac{2\cosh(\lambda)(n+m+1)(n+2)}{(2n+3)} \right. \\
&\left. - a_{n+2}^m c_{n+2}^m(1) \frac{(n+m+1)(n+m+2)}{(2n+3)} \right\} \\
&- \delta_{m1}\Omega_y \times \frac{2n+1}{2n(n+1)} \int_{-1}^{1} \sqrt{\frac{1-\mu^2}{\cosh(\lambda)-\mu}} \sinh(\lambda) N_n^1(\mu)\, d\mu, \qquad (63)
\end{aligned}
$$

with $m = 0$, and $\delta_{m1}$ being the Dirac delta.

## 5.2 Non-axisymmetric components of the velocity coefficients, $m \geq 1$

### 5.2.1 No slip condition at the wall (two equations)

$$
\begin{aligned}
&- \frac{a_{n-1}^m}{2(2n-1)} \frac{B_{n-1}^m}{Co_{n-1}} + \frac{a_{n+1}^m}{2(2n+3)} \frac{B_{n+1}^m}{Co_{n+1}} - \frac{a_{n-1}^{m+1}(n-m-1)}{(2n-1)} \frac{F_{n-1}^m}{Co_{n-1}} \\
&+ a_n^{m+1} \frac{F_n^m}{Co_n} - \frac{a_{n+1}^{m+1}(n+m+2)}{(2n+3)} \frac{F_{n+1}^m}{Co_{n+1}} = 0 \qquad (64)
\end{aligned}
$$

$$
\begin{aligned}
&\frac{a_{n-1}^m (n-m)(n-m+1)}{2(2n-1)} \frac{B_{n-1}^m}{Co_{n-1}} - \frac{a_{n+1}^m (n+m)(n+m+1)}{2(2n+3)} \frac{B_{n+1}^m}{Co_{n+1}} \\
&- \frac{a_{n-1}^{m-1}(n-m+1)}{(2n-1)} \frac{H_{n-1}^m}{Co_{n-1}} - \frac{a_{n+1}^{m-1}(n+m)}{(2n+3)} \frac{H_{n+1}^m}{Co_{n+1}} \\
&+ a_n^{m-1} \frac{H_n^m}{Co_n} = 0 \qquad (65)
\end{aligned}
$$

### 5.2.2 Continuity equation (two equations)

$$
\begin{aligned}
&-\frac{a_{n-1}^{m}\,(n-m)}{2}\frac{B_{n-1}^{m}}{Co_{n-1}}+\frac{5}{2}a_{n}^{m}\frac{B_{n}^{m}}{Co_{n}}+\frac{a_{n+1}^{m}\,(n+m+1)}{2}\frac{B_{n+1}^{m}}{Co_{n+1}}\\
&-a_{n-1}^{m}\,(n-m)\,\frac{C_{n-1}^{m}}{Si_{n-1}}+a_{n}^{m}\,(2n+1)\,\frac{C_{n}^{m}}{Si_{n}}-a_{n+1}^{m}\,(n+m+1)\,\frac{C_{n+1}^{m}}{Si_{n+1}}\\
&-\frac{a_{n-1}^{m+1}}{2}\,(n-m-1)\,(n-m)\,\frac{F_{n-1}^{m}}{Co_{n-1}}+a_{n}^{m+1}\,(n+m+1)\,(n-m)\,\frac{F_{n}^{m}}{Co_{n}}\\
&-\frac{a_{n+1}^{m+1}}{2}\,(n+m+1)\,(n+m+2)\,\frac{F_{n+1}^{m}}{Co_{n+1}}+\frac{a_{n-1}^{m-1}}{2}\frac{H_{n-1}^{m}}{Co_{n-1}}\\
&-a_{n}^{m-1}\frac{H_{n}^{m}}{Co_{n}}+\frac{a_{n+1}^{m-1}}{2}\frac{H_{n+1}^{m}}{Co_{n+1}}=0 \qquad (66)
\end{aligned}
$$

$$
\begin{aligned}
&-\frac{a_{n-1}^{m}\,(n-m)}{2}\frac{A_{n-1}^{m}}{Si_{n-1}}+\frac{5}{2}a_{n}^{m}\frac{A_{n}^{m}}{Si_{n}}+\frac{a_{n+1}^{m}\,(n+m+1)}{2}\frac{A_{n+1}^{m}}{Si_{n+1}}\\
&-\frac{a_{n-1}^{m+1}}{2}\,(n-m-1)\,(n-m)\,\frac{E_{n-1}^{m}}{Si_{n-1}}+a_{n}^{m+1}\,(n+m+1)\,(n-m)\,\frac{E_{n}^{m}}{Si_{n}}\\
&-\frac{a_{n+1}^{m+1}}{2}\,(n+m+1)\,(n+m+2)\,\frac{E_{n+1}^{m}}{Si_{n+1}}+\frac{a_{n-1}^{m-1}}{2}\frac{G_{n-1}^{m}}{Si_{n-1}}\\
&-a_{n}^{m-1}\frac{G_{n}^{m}}{Si_{n}}+\frac{a_{n+1}^{m-1}}{2}\frac{G_{n+1}^{m}}{Si_{n+1}}=0 \qquad (67)
\end{aligned}
$$

### 5.2.3 Slip boundary condition on particle surface (three equations)

In addition to eqn. (63), we have the following:

$$
\begin{aligned}
&-\frac{a_{n-1}^{m}}{2\,(2n-1)}\left(A_{n-1}^{m}+B_{n-1}^{m}\right)+\frac{a_{n+1}^{m}}{2\,(2n+3)}\left(A_{n+1}^{m}+B_{n+1}^{m}\right)\\
&-a_{n-1}^{m+1}\frac{(n-m-1)}{(2n-1)}\left(E_{n-1}^{m}+F_{n-1}^{m}\right)+a_{n}^{m+1}\cosh\left(\lambda\right)\left(E_{n}^{m}+F_{n}^{m}\right)\\
&-a_{n+1}^{m+1}\frac{(n+m+2)}{(2n+3)}\left(E_{n+1}^{m}+F_{n+1}^{m}\right)=\\
&\frac{(2n+1)\,(n-m-1)!}{2\,(n+m+1)!}\sum_{p=m}^{\infty}a_{p}^{m}\left\{\Theta_{np}^{m+1}+\zeta_{np}^{m+1}+\nu_{np}^{m+1}+\kappa_{np}^{m+1}\right\}c_{p}^{m}(1), \qquad (68)
\end{aligned}
$$

and,

$$a_{n-1}^{m}\frac{(n-m)\,(n-m+1)}{2\,(2n-1)}\left(A_{n-1}^{m}+B_{n-1}^{m}\right)-a_{n+1}^{m}\frac{(n+m)\,(n+m+1)}{2\,(2n+3)}\left(A_{n+1}^{m}+B_{n+1}^{m}\right)$$
$$-a_{n-1}^{m-1}\frac{(n-m+1)}{(2n-1)}\left(G_{n-1}^{m}+H_{n-1}^{m}\right)+a_{n}^{m-1}\cosh{(\lambda)}\left(G_{n}^{m}+H_{n}^{m}\right)$$
$$-a_{n+1}^{m-1}\frac{(n+m)}{(2n+3)}\left(G_{n+1}^{m}+H_{n+1}^{m}\right)=$$
$$\frac{(2n+1)(n-m+1)!}{2(n+m-1)!}\sum_{p=m}^{\infty}a_{p}^{m}\left\{\Theta_{np}^{m-1}+\zeta_{np}^{m-1}-\nu_{np}^{m-1}+\kappa_{np}^{m-1}\right\}c_{p}^{m}(1)$$
$$+\delta_{m1}\,(2n+1)\int_{-1}^{1}\sqrt{\cosh{(\lambda)}-\mu}\left\{U_{x}-\Omega_{y}\frac{1-\mu\cosh{(\lambda)}}{\cosh{(\lambda)}-\mu}\right\}N_{n}^{0}\,(\mu)\,d\mu. \qquad (69)$$

In Eq. (68) we have $n\geq m+1$, whereas in Eq. (69) we have $n\geq m-1$. $\delta_{m1}$ in eqn. (69) is the Dirac delta.

In Eqns. (68) and (69), the tensors $\left\{\Theta_{np}^{j},\ \zeta_{np}^{j},\ \kappa_{np}^{j},\ \nu_{np}^{j}\right\}$, with $j=m\pm1$, are integrals involving: (i) the appropriate Legendre polynomials, and, (ii) the dot products of the basis vectors in cylindrical coordinates with those of bi-spherical coordinates (see Eqs. (70) and (71)), as given below.

$$\Theta_{np}^{m\pm1}=\int_{-1}^{1}\frac{\mu\cosh{(\lambda)}-1}{2a}\sqrt{1-\mu^{2}}\frac{N_{n}^{m\pm1}\,(\mu)}{a_{n}^{m\pm1}}\frac{N_{p}^{m}(\mu)}{a_{p}^{m}}d\mu,$$
$$\zeta_{np}^{m\pm1}=\int_{-1}^{1}\left[\frac{\cosh{(\lambda)}-\mu}{2a}\left\{1-\mu\cosh{(\lambda)}\right\}\frac{N_{n}^{m\pm1}\,(\mu)}{a_{n}^{m\pm1}}\times(n+m)(n-m+1)\frac{N_{p}^{m-1}(\mu)}{a_{p}^{m-1}}\right]d\mu, \qquad (70)$$
$$\nu_{np}^{m\pm1}=\int_{-1}^{1}\frac{\left\{\cosh{(\lambda)}-\mu\right\}^{2}}{a\sqrt{1-\mu^{2}}}\frac{N_{n}^{m\pm1}\,(\mu)}{a_{n}^{m\pm1}}\frac{N_{p}^{m}(\mu)}{a_{p}^{m}}d\mu.$$

$$\kappa_{np}^{m\pm1}=\begin{cases}0,\ p=m\\ \int_{-1}^{1}\frac{\cosh(\lambda)-\mu}{2a}\left\{\mu\cosh{(\lambda)}-1\right\}\frac{N_{n}^{m\pm1}(\mu)}{a_{n}^{m\pm1}}\frac{N_{p}^{m+1}(\mu)}{a_{p}^{m+1}}d\mu,\ p\geq m+1\end{cases}. \qquad (71)$$

# References


[1] S. H. Lee and L. G. Leal. Motion of a sphere in the presence of a plane interface. part 2. an exact solution in bipolar co-ordinates. *Journal of Fluid Mechanics*, 98(1):193, May 1980.

[2] N. Desai and S. Michelin. Instability and self-propulsion of active droplets along a wall. *Physical Review Fluids*, 6(11):114103, 2021.

[3] S. Michelin, E. Lauga, and D. Bartolo. Spontaneous autophoretic motion of isotropic particles. *Physics of Fluids*, 25(6):061701, June 2013.

[4] A. Mozaffari, N. Sharifi-Mood, J. Koplik, and C. Maldarelli. Self-diffusiophoretic colloidal propulsion near a solid boundary. *Physics of Fluids*, 28(5):053107, May 2016.
